# Supplementary material for: Mean-field solution of the neural dynamics in a Greenberg-Hastings model with excitatory and inhibitory units
Source: arXiv:2312.17645 source file (2023-12-29)
Supplement: Supplementary file 1 [file supplementary.pdf]

# Supplementary Material of
# Mean-field solution of the neural dynamics in a Greenberg-Hastings model with excitatory and inhibitory units

Joaquin Almeira, Tomas S. Grigera, Daniel A. Martin, Dante R. Chialvo, and Sergio A. Cannas
(Dated: December 29, 2023)

## I. STOCHASTIC TREATMENT

Using the local transition probabilities Eqs.(5) from the main text, we can calculate the transition probabilities for the populations $\vec{\boldsymbol{n}} = (\vec{\boldsymbol{n}}^E, \vec{\boldsymbol{n}}^I) = (n_q^E, n_e^E, n_r^E, n_q^I, n_e^I, n_r^I)$, namely

$$\begin{aligned} U^{E/I}\left(\{n_q^{E/I}, n_e^{E/I}\} \to \{n_q^{E/I}-1, n_e^{E/I}+1\}\right) &= \sum_{q\,\text{state}} (\mu_1 + \alpha\,\Theta) \approx n_q^{E/I}(\mu_1 + \alpha\langle\Theta\rangle) \\ U^{E/I}\left(\{n_e^{E/I}, n_r^{E/I}\} \to \{n_e^{E/I}-1, n_r^{E/I}+1\}\right) &= \sum_{e\,\text{state}} \mu_3 = n_e^{E/I}\mu_3 \\ U^{E/I}\left(\{n_r^{E/I}, n_q^{E/I}\} \to \{n_r^{E/I}-1, n_q^{E/I}+1\}\right) &= \sum_{r\,\text{state}} \mu_2 = n_r^{E/I}\mu_2 \end{aligned} \tag{S1}$$

The approximation made in the first equation $\Theta \to \langle\Theta\rangle$ is expected to be valid for a mean field system. These rates give rise to the Master equation

$$\begin{aligned} \frac{\partial}{\partial t}P(\vec{\boldsymbol{n}}, t) = {}& \mu_3(n_e^E+1)P(n_q^E, n_e^E+1, n_r^E-1, \vec{\boldsymbol{n}}^I, t) + \mu_2(n_r^E+1)P(n_q^E-1, n_e^E, n_r^E+1, \vec{\boldsymbol{n}}^I, t) \\ &+ (\mu_1 + \alpha\langle\Theta\rangle)(n_q^E+1)P(n_q^E+1, n_e^E-1, n_r^E, \vec{\boldsymbol{n}}^I, t) - (\mu_3 n_e^E + \mu_2 n_r^E + (\mu_1+\alpha\langle\Theta\rangle)n_q^E P(\vec{\boldsymbol{n}}, t) \\ &+ (\text{analogous terms for inhibitory}) \end{aligned} \tag{S2}$$

Using a Kramers-Moyal expansion [1] a Fokker-Planck equation for the densities $\vec{\boldsymbol{y}} = \vec{\boldsymbol{n}}/N$ can be derived in the limit $N \to \infty$, namely

$$\frac{\partial}{\partial t}P(\vec{\boldsymbol{y}}, t) = -\sum_i \frac{\partial}{\partial y_i}[a_i P(\vec{\boldsymbol{y}}, t)] + \frac{1}{2}\sum_{ij}\frac{\partial^2}{\partial y_i \partial y_j}[b_{ij}P(\vec{\boldsymbol{y}}, t)] \tag{S3}$$

where subindexes run over six components (three excitatory and three inhibitory) and [1]

$$\begin{aligned} \vec{\boldsymbol{a}} &= (\vec{\boldsymbol{a}}^E, \vec{\boldsymbol{a}}^I) = (a_q^E, a_e^E, a_r^E, a_q^I, a_e^I, a_r^I) = \\ &= (\mathcal{R}^E - \mathcal{Q}^E, \mathcal{Q}^E - \mathcal{E}^E, \mathcal{E}^E - \mathcal{R}^E, \mathcal{R}^I - \mathcal{Q}^I, \mathcal{Q}^I - \mathcal{E}^I, \mathcal{E}^I - \mathcal{R}^I) \end{aligned} \qquad \hat{b} = \begin{pmatrix} \hat{b}^E & 0 \\ 0 & \hat{b}^I \end{pmatrix} \tag{S4}$$

with

$$\hat{b}^{E/I} = \frac{1}{N}\begin{pmatrix} \mathcal{E}^{E/I} + \mathcal{Q}^{E/I} & -\mathcal{Q}^{E/I} & -\mathcal{E}^{E/I} \\ -\mathcal{Q}^{E/I} & \mathcal{Q}^{E/I} + \mathcal{R}^{E/I} & -\mathcal{R}^{E/I} \\ -\mathcal{E}^{E/I} & -\mathcal{R}^{E/I} & \mathcal{E}^{E/I} + \mathcal{R}^{E/I} \end{pmatrix} \begin{matrix} e \\ q \\ r \end{matrix} \quad (\text{columns: } e,\ q,\ r) \qquad \begin{aligned} \mathcal{Q}^{E/I} &= y_q^{E/I}(\mu_1 + \alpha\langle\Theta\rangle) \\ \mathcal{E}^{E/I} &= y_e^{E/I}\mu_3 \\ \mathcal{R}^{E/I} &= y_r^{E/I}\mu_2 \end{aligned} \tag{S5}$$

Under the Itô interpretation [1], we can derive from Eq.(S3) the stochastic differential equation

$$d\vec{\boldsymbol{y}} = \vec{\boldsymbol{A}}(\vec{\boldsymbol{y}}, t)dt + \hat{B}(\vec{\boldsymbol{y}}, t)d\vec{\boldsymbol{\xi}}(t) \tag{S6}$$

where $\vec{\boldsymbol{A}} = (\vec{\boldsymbol{a}}^E, \vec{\boldsymbol{a}}^I)$, $(\hat{B}\hat{B}^{\intercal})_{ij} = b_{ij}$ and $\vec{\boldsymbol{\xi}}$ is a multi-variable Wiener process. Averaging over the noise and defining $\dot{\vec{\boldsymbol{\rho}}} \equiv \langle\dot{\vec{\boldsymbol{y}}}^E\rangle$ and $\dot{\vec{\boldsymbol{\psi}}} \equiv \langle\dot{\vec{\boldsymbol{y}}}^I\rangle$, we obtained

$$
\begin{aligned}
\dot{\rho_q} &= \mu_2\rho_r - (\mu_1 + \alpha\,\langle\Theta\rangle)\rho_q & \qquad \dot{\psi_q} &= \mu_2\psi_r - (\mu_1 + \alpha\,\langle\Theta\rangle)\psi_q \\
\dot{\rho_e} &= (\mu_1 + \alpha\,\langle\Theta\rangle)\rho_q - \mu_3\rho_e & \qquad \dot{\psi_e} &= (\mu_1 + \alpha\,\langle\Theta\rangle)\psi_q - \mu_3\psi_e \\
\dot{\rho_r} &= \mu_3\rho_e - \mu_2\rho_r & \qquad \dot{\psi_r} &= \mu_3\psi_e - \mu_2\psi_r
\end{aligned}
\tag{S7}
$$

Finally, using the relationships

$$
N = N_e + N_i\ , \qquad \rho_e + \rho_q + \rho_r = \frac{N_e}{N} = 1 - f\ , \qquad \psi_e + \psi_q + \psi_r = \frac{N_i}{N} = f
\tag{S8}
$$

we get

$$
\begin{aligned}
\dot{\rho_e} &= (1 - f - \rho_e - \rho_r)\,(\mu_1 + \alpha\langle\Theta\rangle) - \mu_3\rho_e \\
\dot{\rho_r} &= \mu_3\rho_e - \mu_2\rho_r \\
\dot{\psi_e} &= (f - \psi_e - \psi_r)\,(\mu_1 + \alpha\langle\Theta\rangle) - \mu_3\psi_e \\
\dot{\psi_r} &= \mu_3\psi_e - \mu_2\psi_r
\end{aligned}
\tag{S9}
$$

## II. MODEL PARAMETRIZATION

The continuous time stochastic process defined by Eqs.(5) of the main text, can be described as a set of coupled, constant rate jump (or Poisson) processes, each one corresponding to the transition of a single neuron. The Poisson processes are coupled in the sense that an event generated by one process may alter the other process by changing their rates[2]. The transition probabilities of a single neuron $i$ in this continuous time process are then given by [2]

$$
\begin{aligned}
\Pi_i(0 \to 1) &= U_i(0 \to 1)/\nu_i \\
\Pi_i(1 \to 2) &= U_i(1 \to 2)/\nu_i \\
\Pi_i(2 \to 0) &= U_i(2 \to 0)/\nu_i
\end{aligned}
$$

where

$$
\nu_i = U_i(0 \to 1) + U_i(1 \to 2) + U_i(2 \to 0)
$$

Now the basic assumption is that, at least as far as the stationary properties are concerned, the parallel dynamics where the state of all the neurons at time $t+1$ are updated simultaneously from their state at time $t$ (according to the transition probabilities given by Eqs.(5) is equivalent to a sequential update, in a way analogous to the single spin flip rules used in Monte Carlo simulations of discrete spin systems [3]. In other words, neurons in such rules would be updated one by one, where each update may affect the probabilities of the next one. In such a sense, the macroscopic time scale to be compared with the parallel dynamics time unit would be a set of $N$ single update trials (the so-called "Monte Carlo Step"). We checked numerically the stationary properties of both dynamics in different regions of the parameters space for the fully connected model. We verified that both dynamics give qualitatively always the same results, where the quantitative differences become negligible close enough to the dynamical transition regions (not shown). Under the assumption of such equivalency, we can assume that

$$
\Pi_i(0 \to 1) = P_i(0 \to 1) \tag{S10}
$$

$$
\Pi_i(1 \to 2) = P_i(1 \to 2) \tag{S11}
$$

$$
\Pi_i(2 \to 0) = P_i(2 \to 0) \tag{S12}
$$

where the transition probabilities $P_i$ are given by Eqs.(1) of the main text. Hence

$$
\frac{\mu_1 + \alpha\,\Theta}{\nu_i} = 1 - (1 - r_1)(1 - \Theta) \tag{S13}
$$

$$
\frac{\mu_3}{\nu_i} = 1 \tag{S14}
$$

$$
\frac{\mu_2}{\nu_i} = r_2 \tag{S15}
$$

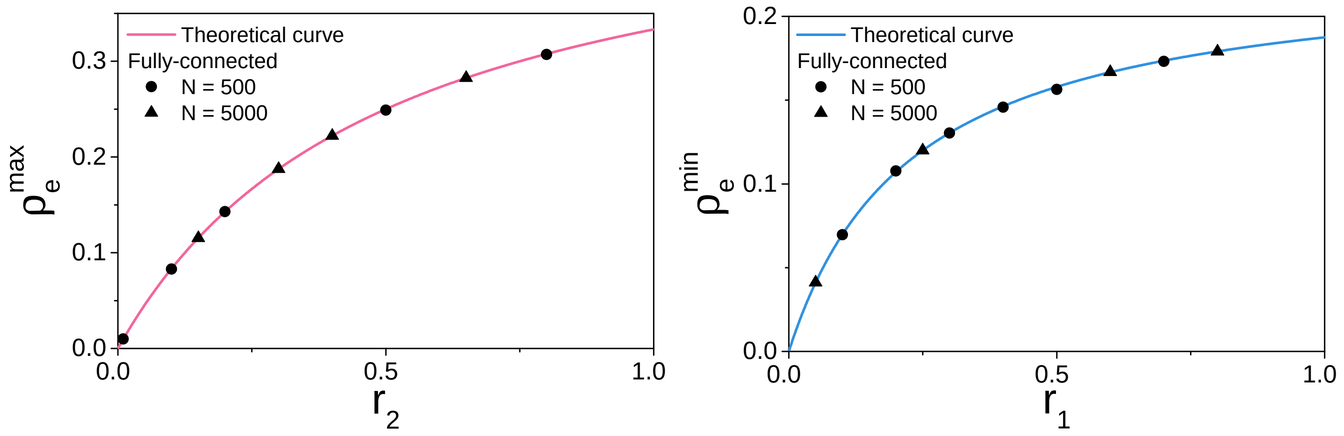


FIG. S1. (a) Maximum activity as a function of $r_2$ for $r_1 = 10^{-3}$ (red solid line). (b) Minimum activity as a function of $r_1$ for $r_2 = 0.3$ (blue solid line). Numerical values of fully connected simulations are plotted for two network sizes in both cases. Theoretical results were obtained for $\sigma^2 = 10^{-7}$

From Eq.(S13) we have that $\mu_1/\nu_i = r_1$ when $\Theta = 0$ and $(\mu_1 + \alpha)/\nu_i = 1$ when $\Theta = 1$. Therefore

$$\mu_1 = \frac{\alpha\, r_1}{1 - r_1} \tag{S16}$$

Combining Eqs.(S14)-(S15) with the last one we obtain

$$\mu_2 = \frac{\alpha\, r_2}{1 - r_1} \tag{S17}$$

$$\mu_3 = \frac{\alpha}{1 - r_1} \tag{S18}$$

Expressions (S16)-(S18) can be checked by considering some limiting cases of f the dynamical equations for $f = 0$:

$$\begin{aligned} \dot{\rho_e} &= (1 - \rho_e - \rho_r)\left(\mu_1 + \eta\left(\frac{\omega\rho_e - T}{\sigma}\right)\right) - \rho_e\mu_3 \\ \dot{\rho_r} &= \rho_e\mu_3 - \rho_r\mu_2 \end{aligned} \tag{S19}$$

As explained in the main text, the stationary solutions of the above equations present a discontinuous transition from a high activity phase to a low activity one as the threshold $T$ is increased, with the presence of hysteresis. The associated maximum ($T \to 0$) and minimum ($T \to \infty$) values of the density of active sites $\rho_e$ correspond to the stationary solutions Eqs.(S19) when $\eta \to 0$ and $\eta \to 1$ respectively. Combining such solutions with Eqs.(S16)-(S18)(assuming $\alpha = 1$, see manuscript) we obtain the expressions

$$\rho_e^{min} = \frac{r_2}{2r_2 + 1} \qquad\qquad \rho_e^{max} = \frac{1}{1 + 1/r_1 + 1/r_2}, \tag{S20}$$

which are independent of $\sigma$ and therefore from the system size. These can be compared with numerical simulation results from the microscopic model. The comparison shown in Fig.S1 exhibits a full agreement in the whole range of values of $r_1$ and $r_2$

## III. FINITE SIZE SCALING

We analysed the finite size scaling of the variance $\sigma^2 = \langle v_i^2\rangle - \langle v_i\rangle^2$ for the microscopic model defined on a fully connected network with $N$ sites, where the variables $v_i$ are defined as

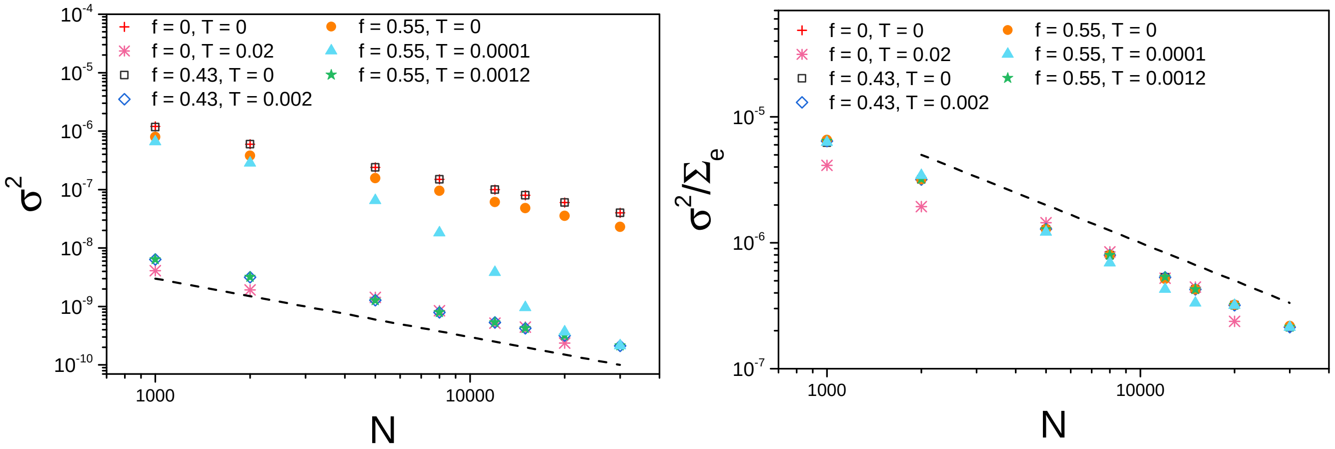


FIG. S2. Finite size scaling of the variance $\sigma^2$ for different combinations of the parameters $(f, T)$. Left: $\sigma^2$ as a function of $N$. Right: $\sigma^2/\Sigma_e$ as a function of $N$. The dashed lines are power laws $N^{-1}$.

$$v_i = \frac{1}{N}\sum_{j=1}^{N} w_{ij}\epsilon_j \delta(x_j(t), 1) - T. \tag{S21}$$

The averages are taken over a single run of the dynamics and over the quenched disorder variables $w_{ij}$ and $\epsilon_i$, It is assumed that $\sigma$ is independent of the site $i$. The results are shown in Fig.S2, for different values of the parameters $(f, T)$. We see, that in all cases $\sigma^2 \propto C/N$, where $C \propto \Sigma_e$ (See Fig.S3).

## IV. HYSTERESIS

To verify the existence of hysteresis we solved numerically the dynamical equations for $f = 0$

$$\begin{aligned} \dot{\rho_e} &= (1 - \rho_e - \rho_r)\left(\mu_1 + \eta\left(\frac{\omega\rho_e - T}{\sigma}\right)\right) - \rho_e\mu_3 \\ \dot{\rho_r} &= \rho_e\mu_3 - \rho_r\mu_2, \end{aligned} \tag{S22}$$

with constant values of $\sigma$. We verified that for small enough values of $\sigma$ the properties of the stationary state of Eqs.(S22) are almost insensitive to $\sigma$ for a wide range (around two orders of magnitude) of values of it. We performed a loop of increasing-decreasing $T$ and solving Eqs.(S22) using the Runge-Kutta (RK) method. For each value of $T$, we run the RK algorithm until the system reaches a stationary state and record the stationary value of $\rho_e$ before changing $T \to T \pm \Delta T$ ($\Delta T \sim 1.5 \times 10^{-5}$) and restart the RK algorithm with the previous state as the new initial condition. We also performed a similar loop in a numerically simulated GH model in a fully connected network. In this case, for every value of $T$, we discard the first $t = 500$ steps and average the fraction of active sites over $10^3 - 10^4$ steps before changing $T$, taking the last configuration as the initial one for the new value of $T$. In Fig.S3 we compare two loops of $\rho_e$ *vs.* $T$ for both systems, one with $N = 30000$ and the other with $\sigma = 10^{-4}$. We also show the hysteresis width $\Gamma$[4] as a function of the network size $N$ for numerical simulated GH model loops or as a function of $\sigma$ for numerical solutions of the Eqs.(12). We find that $\Gamma$ converges through a power law to its limit value $\Gamma_{max} = T_{max} - T_{min}$ for $N \to \infty$ and $\sigma \to 0$ in each case, where $T_{min}$ and $T_{max}$ are given by Eqs.(24) of main text.

## V. UNSTABLE SOLUTION

We considered here the case $f = 0$. The unstable solution in the general case can be derived in a similar way.

In the limit $\sigma \to 0$, $\eta(\frac{\omega\rho_e - T}{\sigma})$ can only have 3 values: 0, 1, and 1/2. The first two correspond to stable solutions. We found that the third one is close to the unstable solution presented by the model. To find that solution, we

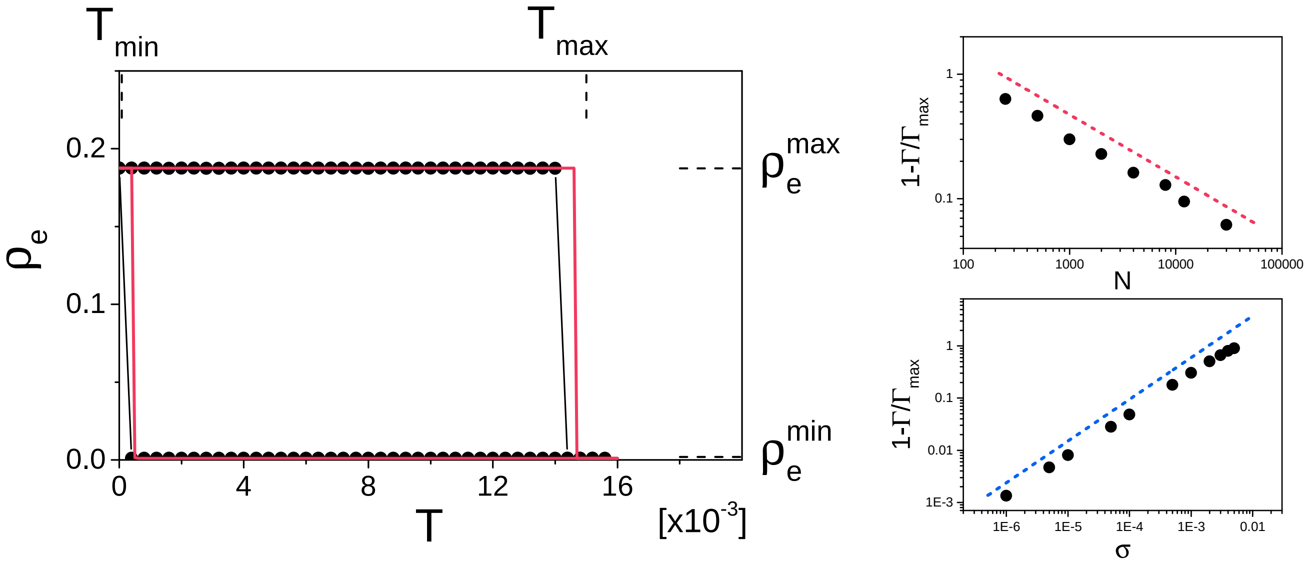


FIG. S3. Left: Comparison between a hysteresis loop generated with Greenberg-Hastings dynamics over a fully connected network of size $N = 30000$ (black line-dots) and one obtained from the mean-field model with parameter $\sigma = 10^{-4}$ (solid pink line). Right: Hysteresis width $\Gamma$ tends to its maximum value $\Gamma_{max}$ in the thermodynamic limit ($N \to \infty$ or $\sigma \to 0$) as power law for both models. The pink dashed line is a power law in the network size $\sim N^{-0.5}$ while the blue dashed line is a power law in the $\sigma$ parameter $\sim \sigma^{0.8}$.

approximated $\eta(x)$ by the first two terms of its Taylor series expansion, $\frac{1}{2}(1+x)$, obtaining the equation for the stationary solution:

$$\left(1 - \rho_e(1 + \frac{\mu_3}{\mu_2})\right) \cdot \left(\mu_1 + \frac{1}{2} + \frac{\omega\rho_e - T}{2\sigma}\right) - \rho_e\mu_3 = 0 \tag{S23}$$

This is second degree polynomial on $\rho_e$. It has 2 solutions, one for which $\rho_e > \rho_e^{max}$, and the other, which is close to $\frac{T}{\omega}$. This solution is already plotted in Fig. 2 of the main text.

## VI. STABILITY OF $\Delta_{e/r} = 0$

The equations for $\Delta_{e/r}$ are:

$$\dot{\Delta}_e = (-\mu_3 - \mathcal{N})\Delta_e - \mathcal{N}\Delta_r \tag{S24a}$$

$$\dot{\Delta}_r = \mu_3\Delta_e - \mu_2\Delta_r. \tag{S24b}$$

In the stationary state, the equations for $\Delta_{e/r}$ read:

$$(-\mu_3 - \mathcal{N})\Delta_e^* - \mathcal{N}\Delta_r^* = 0$$

$$\mu_3\Delta_e^* - \mu_2\Delta_r^* = 0 \tag{S25a}$$

Since we are in the stationary state $\mathcal{N}$ is constant. Hence, we can consider the above system as two linear equations on $\Delta_{e/r}$. Both equations are linearly independent since the first one has 2 negative coefficients and the second one has one positive and the other negative. Then, they have only one solution, which is $\Delta_{e/r}^* = 0$ (for any value of $\mathcal{N}$). We now consider their stability. We can write

$$\Delta_{e/r} = \Delta_{e/r}^* + \delta\Delta_{e/r} \tag{S26}$$

$$\Sigma_{e/r} = \Sigma_{e/r}^* + \delta\Sigma_{e/r}, \tag{S27}$$

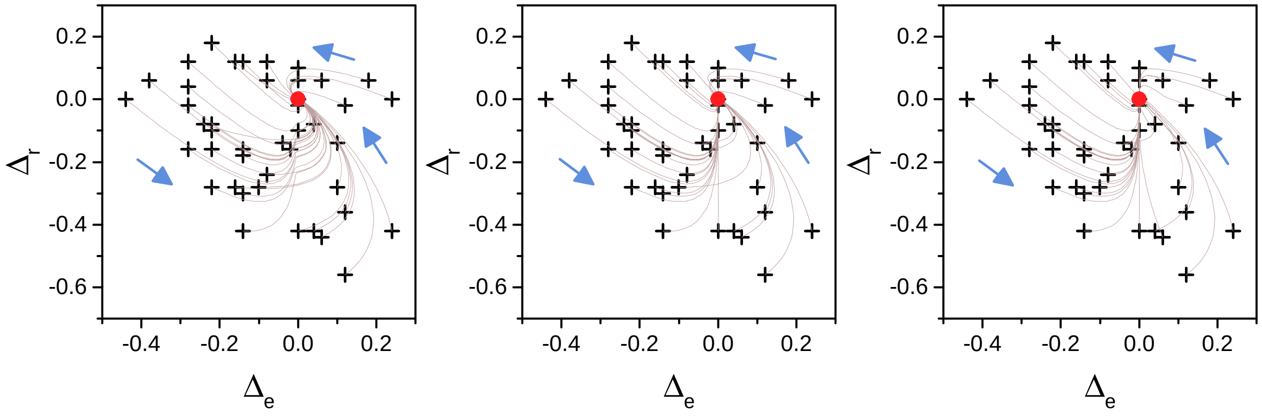


FIG. S4. Evolution of $\Delta_e$ and $\Delta_r$ computed the from full system of equations, Eqs.(12) for different parameters and initial conditions. The trajectories for $\Delta_r$ as a function of $\Delta_e$ are shown for $f = 0.3$, and 3 values of $T$: $T = 0$ (left), $T = 0.004$ (middle) and $T = 0.02$ (right). We computed trajectories for all the possible combinations of the following initial values: $\rho_e = 0$, 0.2, ..., 1; $\rho_r = 0$, 0.2, ..., $1 - \rho_e$; $\psi_e = 0$, 0.2, ..., 1; and $\psi_r = 0$, 0.2, ..., $1 - \psi_e$, making a total of 225 trajectories for each value of $T$. For clarity, we only show approximately 20% of the trajectories, randomly selected. Black crosses correspond to different initial conditions and the red circles correspond to the final conditions. The arrows show the instantaneous evolution of a few selected trajectories. Notice that different combinations of $\rho_{e/r}$ and $\psi_{e/r}$ may lead to the same values of $\Delta_{e/r}$

where $\delta\Sigma_{e/r}$ and $\delta\Delta_{e/r}$ are the (small) fluctuations of $\Delta_{e/r}$ and $\Sigma_{e/r}$ around their stationary values. We can also write $\mathcal{N} = \mathcal{N}^* + \delta\mathcal{N}$, with $\delta\mathcal{N} = \frac{\partial\mathcal{N}}{\partial\Sigma_e}\delta\Sigma_e + \frac{\partial\mathcal{N}}{\partial\Delta_e}\delta\Delta_e$. We then get:

$$\delta\dot{\Delta}_e = (-\mu_3 - \mathcal{N}^*)\delta\Delta_e - \delta\mathcal{N}\underbrace{\Delta_e^*}_{0} - \mathcal{N}^* + \delta\Delta_r - \delta\mathcal{N}\underbrace{\Delta_r^*}_{0} + O(\delta^2)$$
$$\delta\dot{\Delta}_r = \mu_3\delta\Delta_e - \mu_2\delta\Delta_r + O(\delta^2) \tag{S28}$$

This can be written in matrix form:

$$\begin{pmatrix} \delta\dot{\Delta}_e \\ \delta\dot{\Delta}_R \end{pmatrix} = \begin{pmatrix} -\mu_3 - \mathcal{N}^* & -\mathcal{N}^* \\ \mu_3 & -\mu_2 \end{pmatrix} \cdot \begin{pmatrix} \delta\Delta_e \\ \delta\Delta_R \end{pmatrix},$$

The eigenvalues of the matrix are $\lambda_\pm = \frac{-\mathcal{N}*-\mu_3-\mu_2}{2} \pm \frac{1}{2}\sqrt{(\mathcal{N}^* - \mu_3 - \mu_2)^2 - 4\mu_2\mu_3}$, which have negative real part, so the solution is stable. We have computed numerically the evolution of the $\rho_{e/r}$ and $\psi_{e/r}$, Eqs.(12), for different values of $f$ and $T$, and several different initial conditions. The results show that the different trajectories converge to $\Delta_{e/r} = 0$. In Fig.S4 we show some examples of these trajectories for $f = 0.3$, and three values of $T$: $T = 0$ (where the only stationary solution corresponds to $\Sigma_e \simeq \Sigma_e^{max}$), $T = 0.004$ (where $\Sigma_e \simeq \Sigma_e^{max}$ and $\Sigma_e \simeq \Sigma_e^{min}$ coexist), and $T = 0.02$ (where $\Sigma_e \simeq \Sigma_e^{min}$).

[1] C. Gardiner, *Stochastic Methods, A Handbook for the Natural and Social Sciences* (Springer Series in Synergetics), Springer Berlin, Heidelberg, (2009).
[2] N Masuda, C Vestergaard, *Gillespie Algorithms for Stochastic Multiagent Dynamics in Populations and Networks* (Elements in the Structure and Dynamics of Complex Networks), Cambridge: Cambridge University Press, (2023).
[3] D. P. Landau and K. Binder, *Monte-Carlo Simulations in Statistical Physics*, Cambridge University press (2009)
[4] The hysteresis width Γ is calculated as the difference between the threshold values in the loop edges. Those thresholds are an average between the values in the upper and lower corners of the loop edges.
